# Supplementary material for: A Global Perspective on the Past, Present, and Future of Video Streaming over Starlink
Source: arXiv:2409.09846 source file (2024-09-15)
Supplement: Supplementary file 1 [file appendix.tex]

\appendix
\section{Ethics}
